# Supplementary material for: Generative AI Practices, Literacy, and Divides: An Empirical Analysis in the Italian Context
Source: arXiv:2512.03671 source file (2026-05-19)
Supplement: Supplementary file 1 [file supplementary.pdf]

# Supplementary Materials

## S1 Experimental Details

### S1.1 LT and GenAI Chatbot Definitions

The definitions and examples of each language technology in our survey are provided in Table [S1](#).

### S1.2 List of GenAI Activities

In the following, we provide a full list of the 26 GenAI activities (translated to English) included in the survey.

- **Conversations and Support**
  - Medical advice
  - Personal advice
  - Emotional or psychological support
  - Other advice and suggestions
  - Friendly conversations
  - Philosophical or political conversations
  - Romantic or erotic conversations
  - Other conversations
- **Generation and Content Creation**
  - Quiz creation
  - Audio or music generation
  - Image generation
- **Writing and Analysis**
  - Analysis (general)
  - Data analysis and comprehension
  - Programming language assistance
  - Summaries
  - Academic writing
  - Creative writing
  - Email writing
  - Other writing
- **Others**
  - Travel and itinerary planning
  - Idea collection and draft creation
  - Explanations
  - Text comprehension and formatting

| Item                                 | Definition                                                                                                                                                                                                        | Examples                                                                                                   |
|--------------------------------------|-------------------------------------------------------------------------------------------------------------------------------------------------------------------------------------------------------------------|------------------------------------------------------------------------------------------------------------|
| <i>General Definition</i>            |                                                                                                                                                                                                                   |                                                                                                            |
| Language Technologies                | Tools based on artificial intelligence (AI) used to analyze and produce human language, both written and spoken.                                                                                                  | Voice assistants, machine translators, voice generation, assisted writing, speech transcript, chatbots     |
| <i>Task-Specific LT Applications</i> |                                                                                                                                                                                                                   |                                                                                                            |
| Machine Translation                  | Applications that automate the translation of text or speech from one language to another.                                                                                                                        | Google Translate, DeepL, Microsoft Bing, Amazon Translator                                                 |
| Voice Assistants                     | Applications designed to perform tasks, provide information, and control devices through voice commands.                                                                                                          | Siri, Google Assistant, Alexa, Cortana, Bixby, Celia                                                       |
| Assisted Writing                     | Applications for text correction and revision (grammar, paraphrasing, and summarizing), or support for creative writing. It does not include generating text from scratch, only revision of already drafted text. | Grammarly, Writefull, QuillBot, Smart Compose (Google), Jasper AI                                          |
| Speech Transcription                 | Applications for transcribing audio content into text, such as dictation systems, subtitling tools, or applications for the hearing impaired.                                                                     | Apple Note, Automatic transcription on Zoom / Google Meet / Teams, Otter.AI, Speechmatics, Rev             |
| Text-to-Speech                       | Applications for generating artificial voice and reading text aloud.                                                                                                                                              | Google Cloud Text-to-speech, IBM Watson, ElevenLabs, Adobe Acrobat Read Aloud, Apple VoiceOver, NVDA, JAWS |
| <i>General-Purpose GenAI Systems</i> |                                                                                                                                                                                                                   |                                                                                                            |
| Chatbots                             | General-purpose systems for creating text, images, audio, or other content from simple verbal prompts. Allow natural interaction via chat to obtain answers, support, or complete various tasks.                  | ChatGPT, Gemini, Claude, Copilot, Perplexity                                                               |

**Table S1** Definitions and examples of language technologies.

| Method  | Parameter        | Language Choice | Modality Type |
|---------|------------------|-----------------|---------------|
| UMAP    | n_neighbors      | 10              | 5             |
|         | n_components     | 20              | 20            |
| HDBSCAN | min_cluster_size | 10              | 6             |
|         | min_samples      | 5               | 5             |

**Table S2 BERTopic parameters.** Final choice for UMAP and HDBSCAN parameters for the open-text questions about users’ expressed preference about the language chosen to prompt the model and the modality, i.e., typing or speaking.

- Fact checking (verification of information accuracy)

### S1.3 Demographic Sample

To compare our demographic sample, in Figure S2 we plot the population of our survey (teal bars) compared to the national one (red dashed reference lines). For representative values and distribution, we refer to the Italian National Institute of Statistics (ISTAT) 2025 data (<https://demo.istat.it/app/?i=POS&l=it>). Values are reported as percentages across four key demographic categories, i.e., gender, age, geographic area, and education.

### S1.4 BERTopic Details and Configuration

BERTopic is Python software<sup>1</sup> commonly used for topic modeling. Off-the-shelf, it offers an integrated interface to a wide range of natural language processing tools, along with high customizability.

Our BERTopic processing pipeline includes several steps. First, it converts each text individually into a numerical representation. For this step, we used a state-of-the-art *sentence embedder* model, namely Qwen3-Embedding-8B (Zhang et al. 2025). Sentence embedders capture semantic meaning in a format suitable for computational analyses by computing an N-dimensional vector representation for the text, also known as *embedding*. The geometrical properties of embeddings are commonly used for semantic search and information retrieval (e.g., the cosine similarity between embeddings is often used to retrieve documents relevant to a user query). Second, BERTopic applies dimensionality reduction using UMAP (McInnes et al. 2018) to minimize noise by reducing the embedding dimensionality. Third, it uses the HDBSCAN clustering algorithm (McInnes et al. 2017) to group semantically similar responses. In all cases, this step produced no more than 25 distinct clusters. Finally, for each cluster, the algorithm selects the N most relevant texts and compiles a prompt for a large language model. For this step, we prompted Gemma 3 Instruct (Team et al. 2025), a leading generative language model, to provide a detailed but concise summary of the cluster’s topics. Listing S1 reports the prompt we used. Since some textual nuances introduce noise, we manually verified all extracted clusters and merged similar ones.

Before running the BERTopic pipeline, we exclude all responses shorter than three characters and remove a set of Italian stopwords as found at <https://github.com/>

```

I wrote and published a survey to understand how Italians use generative AI.
→ The survey and the participant responses are in Italian.
Now, I am analyzing the following open-form question:

# Question
[question]

After clustering my answers, I have identified a topic described by the
→ following keywords.

# Keywords
[keywords]

The following responses are a representative sample of the cluster
→ representing the topic

# Documents
[documents]

# Guidelines
Based on this information, your task is to generate a topic description in
→ the context of this question. Here are the guidelines:
1. The description must be detailed and exhaustive, but it CANNOT exceed 300
→ words.
2. Describe what brought you to the description by mentioning the sample
→ answers.
3. Do not mention the question, it's known to the reader. Moreover, do not
→ make any assumption of the number of responses in the cluster.
4. Begin the description with a short title that summarizes it, e.g.,
→ "Enhanced perceived precision. <description>", or "Chosen due to
→ convenience. <description>"
5. If the answers are simply "no" or "nessuna", this is a cluster with
→ negative answers. In this case, just avoid spending many words and say
→ "Negative answers".

Begin the answer right after this prompt.

```

**Fig. S1 Cluster summarization prompt.** [question], [keywords], and [documents] are replaced with one of the questions of the survey, the 10 most relevant keywords and documents describing the cluster, respectively.

[stopwords-iso/stopwords-it/blob/master/stopwords-it.txt](https://stopwords-iso.github.io/stopwords-it/blob/master/stopwords-it.txt) from the remaining ones. We manually tuned two UMAP and HDBSCAN parameter sets to adjust cluster granularity and diversity based on the question. Table S2 reports all the final parameters.

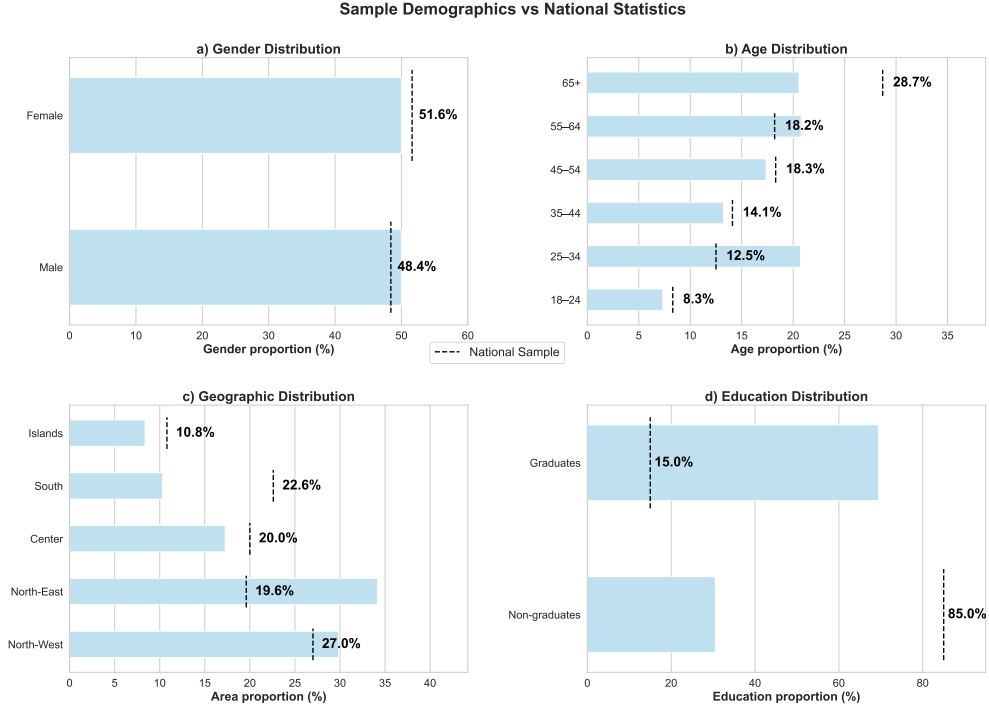

**Fig. S2** Distribution of demographic characteristics in our sample (teal bars) relative to national statistics (red dashed reference lines), broken down by (a) gender, (b) age, (c) geographic area, and (d) education.

## S2 Additional Results

### S2.1 Sample Robustness Checks

To assess the robustness of our findings, we applied post-stratification weights based on Italian population benchmarks from ISTAT 2025 data for gender, age, and geography. We computed frequency tables comparing unweighted and weighted percentages across all key variables, calculating the delta ( $\Delta$ ; difference in percentage points) for each categorical response. We classified variables using three thresholds based on the maximum delta across categories: *pass* ( $\Delta \leq 3$  pp), *review* ( $3 < \Delta \leq 5$  pp), and *critical* ( $\Delta > 5$  pp). We also verified whether the top-2 responses remained consistent between weighted and unweighted distributions.

Most key variables showed minimal weighting effects. Educational level and socioeconomic status all passed the robustness check with deltas under 2 pp. GenAI chatbot adoption (80.4% vs. 80.1% weighted), language technology usage and replacement behaviors were similarly robust. Usage modalities, strategies, and prior experiences with errors also showed stable patterns. Intent frequencies for using GenAI passed checks with deltas under 2.5 pp, with the sole exception of the “Learning” intent, where weighted estimates showed slightly higher weekly use ( $\Delta = 3.02$  pp).

| Variable        | VIF   | Df | VIF (Norm) |
|-----------------|-------|----|------------|
| Age Group       | 1.178 | 1  | 1.086      |
| Education Group | 1.077 | 1  | 1.038      |
| Gender Group    | 1.033 | 1  | 1.016      |
| Geography Group | 1.013 | 2  | 1.003      |
| Income Group    | 1.074 | 1  | 1.036      |
| LT Experience   | 1.130 | 1  | 1.063      |
| LT Literacy     | 1.167 | 1  | 1.080      |

**Table S3 Variance Inflation Factors (VIF).**

Values for each predictor variable in our study, degree of freedom (Df), and normalized VIF (Norm) obtained as  $VIF^{1/2 \cdot Df}$ .

All substantive directions remained consistent, and only two sets of responses exhibited larger weighting effects. English language use showed a 5.06 pp delta, with weighted samples showing higher adoption (53.4% vs. 48.4%), potentially reflecting over-representation of younger respondents. Work versus personal use patterns varied by occupation, with Healthcare ( $\Delta = 15.25$  pp) and Services and Hospitality ( $\Delta = 5.61$  pp) flagged as *critical*, likely due to small subcategory sample sizes ( $n = 74$  and  $n = 35$  respectively), but while keeping the overall trends unchanged.

Overall, our main findings regarding demographic disparities, adoption patterns, and replacement behaviors remain robust to post-stratification weighting, supporting our decision to report unweighted results and retain all participant responses.

## S2.2 Multi-collinearity Verification

Multi-collinearity between predictor variables may hinder the reliability of regression analyses. Across our experiments, we use seven variables divided into numerical, ordinal, and categorical: Education Group (categorical), Geography Group (categorical), Gender Group (categorical), Socioeconomic Group (ordinal), Age Group (ordinal), LT Experience (numerical), and LT Literacy (numerical).

To verify multi-collinearity, we follow a standard approach based on Variance Inflation Factors (VIF; O’Brien 2007). Specifically, we use linear regression and  $R^2$  to estimate numerical variables and logistic-type models and McFadden’s pseudo- $R^2$  for categorical and ordinal ones. Table S3 reports the VIF value for each variable. The highest score is 1.178, indicating a non-problematic multicollinearity.

## S2.3 Modeling

Table S5 reports the Odds Ratios and Standard Errors for GenAI chatbot usage across demographic, socioeconomic, geographic, and language technology factors, while Table S6 presents the OLS Regression coefficients of the frequency of use by GenAI chatbot users for each use intent.

| Language | %    | Modality                  | %    |
|----------|------|---------------------------|------|
| Italian  | 95.3 | Mainly writing            | 84.6 |
| English  | 51.5 | Both writing and speaking | 13.2 |
| Other    | 5.2  | Mainly speaking           | 2.2  |

**Table S4 Results for language usage and interaction modality.** Percentage and count of responses to the multiple-choice question “*In which language do you interact with chatbots?*” and the single-choice answers to “*Which interaction modality do you use?*”.

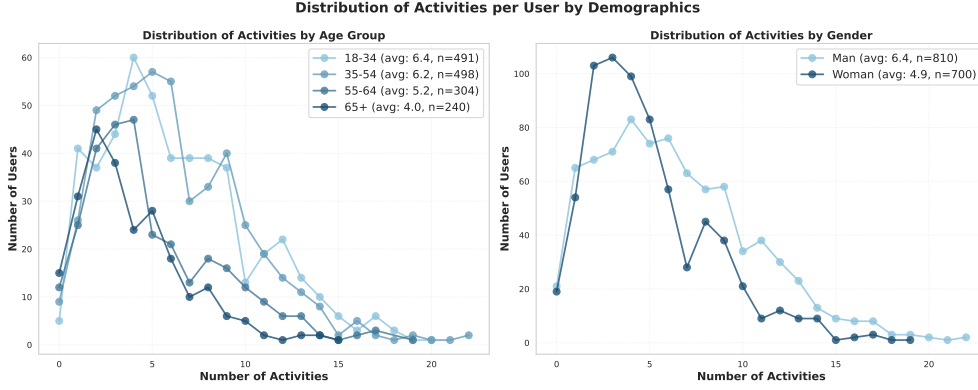

**Fig. S3 Distribution of the number of different activities performed with GenAI chatbots across gender and age groups.** Age groups on the *left*, gender groups on the *right*.

## References

- McInnes L, Healy J, Astels S, et al (2017) hdbscan: Hierarchical density based clustering. J Open Source Softw 2(11):205
- McInnes L, Healy J, Melville J (2018) Umap: Uniform manifold approximation and projection for dimension reduction. arXiv preprint arXiv:180203426
- O’Brien RM (2007) A caution regarding rules of thumb for variance inflation factors. Quality & quantity 41(5):673–690
- Team G, Kamath A, Ferret J, et al (2025) Gemma 3 technical report. URL <https://arxiv.org/abs/2503.19786>, arXiv:2503.19786
- Zhang Y, Li M, Long D, et al (2025) Qwen3 Embedding: Advancing Text Embedding and Reranking Through Foundation Models. arXiv preprint arXiv:250605176

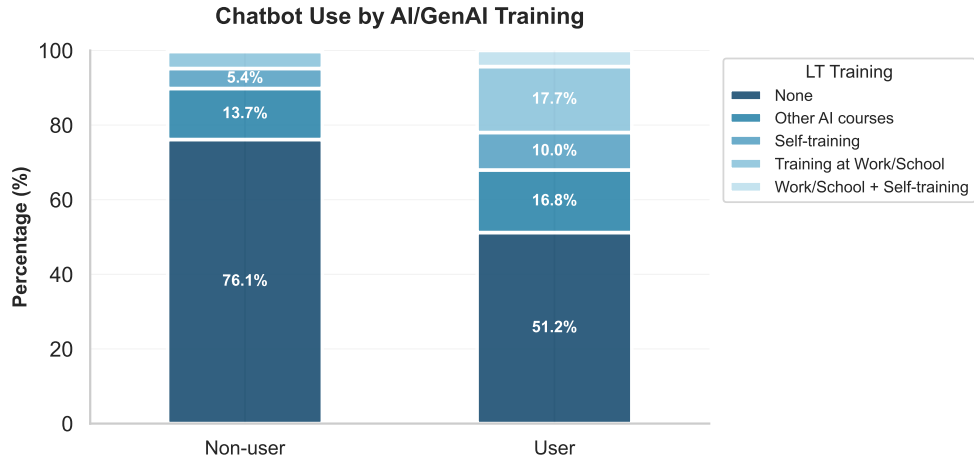

**Fig. S4 Prior training in LT by chatbot usage status.** Respondents were asked whether they had received prior training in AI-based LT technology via both formal or informal channels. Among chatbot users ( $n = 1,542$ ), 51.2% reported no prior training, while 76.2% of non-users ( $n = 373$ ) had no training background at all. Users showed higher rates of formal training through work/school (16.8% vs. 0%), as well as combined formal and self-training (17.6% vs. 5.2%). A small proportion in both groups reported other AI-related coursework (User: 10.1%, Non-user: 13.6%).

| Variable                             | Odds Ratio | Standard Error |    |
|--------------------------------------|------------|----------------|----|
| Gender: Woman (Man)                  | 0.501      | 0.071          | ** |
| Age: 35-54 (18-34)                   | 0.437      | 0.098          | ** |
| Age: 55-64 (18-34)                   | 0.370      | 0.085          | ** |
| Age: 65+ (18-34)                     | 0.196      | 0.044          | ** |
| Geography: Centre (North)            | 1.077      | 0.205          |    |
| Geography: South&Islands (North)     | 0.817      | 0.150          |    |
| Geography: Abroad (North)            | 0.817      | 0.284          |    |
| Income: Mid (Lower)                  | 1.322      | 0.239          |    |
| Income: Higher (Lower)               | 1.726      | 0.375          | ** |
| Education: Graduates (Non-graduates) | 1.482      | 0.219          | ** |
| LT experience                        | 1.715      | 0.130          | ** |
| LT literacy                          | 20.819     | 7.001          | ** |

**Table S5** Odds Ratios and Standard Errors for GenAI chatbot usage across demographic, socioeconomic, geographic, and language technology factors. Reference categories are shown in parentheses, and statistically significant results are indicated with \*\*.



|                      | Information          | Problem              | Learning             | Content              | Leisure              | Creativity           |
|----------------------|----------------------|----------------------|----------------------|----------------------|----------------------|----------------------|
| <b>Age</b>           |                      |                      |                      |                      |                      |                      |
| 35-54                | 0.151**<br>(0.074)   | -0.016<br>(0.071)    | -0.085<br>(0.069)    | 0.085<br>(0.070)     | -0.022<br>(0.068)    | -0.051<br>(0.070)    |
| 55-64                | 0.206**<br>(0.086)   | -0.054<br>(0.082)    | -0.184**<br>(0.081)  | -0.190**<br>(0.082)  | -0.001<br>(0.080)    | -0.183**<br>(0.082)  |
| 65+                  | 0.328***<br>(0.098)  | -0.002<br>(0.095)    | -0.074<br>(0.092)    | -0.657***<br>(0.094) | -0.047<br>(0.092)    | -0.270***<br>(0.094) |
| <b>Education</b>     |                      |                      |                      |                      |                      |                      |
| Graduates            | 0.070<br>(0.069)     | -0.030<br>(0.066)    | -0.086<br>(0.064)    | 0.248***<br>(0.066)  | -0.112*<br>(0.064)   | -0.080<br>(0.065)    |
| <b>Gender</b>        |                      |                      |                      |                      |                      |                      |
| Woman                | -0.220***<br>(0.061) | -0.376***<br>(0.058) | -0.312***<br>(0.057) | -0.097*<br>(0.058)   | -0.286***<br>(0.056) | -0.140**<br>(0.058)  |
| <b>Geography</b>     |                      |                      |                      |                      |                      |                      |
| Abroad               | -0.004<br>(0.126)    | 0.190<br>(0.120)     | 0.064<br>(0.118)     | 0.267**<br>(0.120)   | -0.095<br>(0.116)    | 0.022<br>(0.119)     |
| Centre               | 0.101<br>(0.082)     | 0.116<br>(0.079)     | 0.036<br>(0.077)     | 0.051<br>(0.078)     | 0.127*<br>(0.076)    | 0.111<br>(0.078)     |
| South& Islands       | -0.023<br>(0.082)    | 0.037<br>(0.078)     | 0.114<br>(0.077)     | 0.147*<br>(0.077)    | 0.133*<br>(0.076)    | -0.022<br>(0.077)    |
| <b>Income</b>        |                      |                      |                      |                      |                      |                      |
| Higher               | 0.221**<br>(0.091)   | 0.087<br>(0.088)     | 0.273***<br>(0.086)  | 0.214**<br>(0.087)   | -0.069<br>(0.084)    | 0.197**<br>(0.087)   |
| Mid                  | 0.044<br>(0.082)     | 0.032<br>(0.078)     | 0.083<br>(0.077)     | 0.034<br>(0.078)     | -0.180**<br>(0.075)  | 0.023<br>(0.078)     |
| <b>LT experience</b> |                      |                      |                      |                      |                      |                      |
|                      | 0.032<br>(0.029)     | 0.073***<br>(0.028)  | 0.035<br>(0.027)     | 0.149***<br>(0.028)  | 0.045*<br>(0.027)    | 0.146***<br>(0.028)  |
| <b>LT literacy</b>   |                      |                      |                      |                      |                      |                      |
|                      | 0.008<br>(0.148)     | 0.449***<br>(0.141)  | 0.357***<br>(0.138)  | 0.944***<br>(0.140)  | 0.340**<br>(0.137)   | 0.413***<br>(0.140)  |
| Intercept            | 1.794***<br>(0.146)  | 1.695***<br>(0.140)  | 1.940***<br>(0.137)  | 0.853***<br>(0.139)  | 0.718***<br>(0.134)  | 0.923***<br>(0.138)  |
| Observations         | 1407                 | 1385                 | 1401                 | 1388                 | 1350                 | 1385                 |
| $R^2$                | 0.034                | 0.057                | 0.048                | 0.164                | 0.045                | 0.059                |
| Adjusted $R^2$       | 0.026                | 0.049                | 0.040                | 0.157                | 0.036                | 0.051                |

Note:

\*p<0.1; \*\*p<0.05; \*\*\*p<0.01

**Table S6 OLS Regression coefficients of the frequency of use of GenAI chatbots.** We run six OLS models, one per intent (columns). Standard Errors are reported between parentheses.

|                      | Information        | Problem            | Learning           | Content             | Leisure           | Creativity         |
|----------------------|--------------------|--------------------|--------------------|---------------------|-------------------|--------------------|
| <b>Age</b>           |                    |                    |                    |                     |                   |                    |
| 35-54                | 1.327**<br>(.17)   | 1.024<br>(.129)    | .901<br>(.115)     | 1.211<br>(.158)     | .911<br>(.119)    | .953<br>(.114)     |
| 55-64                | 1.461**<br>(.216)  | .946<br>(.135)     | .76*<br>(.113)     | .738**<br>(.108)    | .906<br>(.147)    | .738**<br>(.107)   |
| 65+                  | 1.716***<br>(.281) | 1.035<br>(.176)    | .908<br>(.154)     | .345***<br>(.058)   | .866<br>(.164)    | .633***<br>(.106)  |
| <b>Education</b>     |                    |                    |                    |                     |                   |                    |
| Graduates            | 1.103<br>(.131)    | .946<br>(.11)      | .846<br>(.102)     | 1.501***<br>(.185)  | .849<br>(.109)    | .872<br>(.102)     |
| <b>Gender</b>        |                    |                    |                    |                     |                   |                    |
| Woman                | .679***<br>(.072)  | .507***<br>(.053)  | .583***<br>(.061)  | .883<br>(.094)      | .541***<br>(.062) | .809***<br>(.081)  |
| <b>Geography</b>     |                    |                    |                    |                     |                   |                    |
| Abroad               | .991<br>(.207)     | 1.45*<br>(.322)    | 1.046<br>(.194)    | 1.665***<br>(.43)   | .825<br>(.184)    | 1.017<br>(.217)    |
| Centre               | 1.216<br>(.174)    | 1.253<br>(.185)    | 1.077<br>(.157)    | 1.096<br>(.157)     | 1.329**<br>(.191) | 1.2<br>(.173)      |
| South& Islands       | .992<br>(.149)     | 1.084<br>(.151)    | 1.311*<br>(.197)   | 1.229<br>(.172)     | 1.281<br>(.196)   | .96<br>(.125)      |
| <b>Income</b>        |                    |                    |                    |                     |                   |                    |
| Higher               | 1.453**<br>(.232)  | 1.184<br>(.184)    | 1.619***<br>(.265) | 1.457**<br>(.231)   | .837<br>(.138)    | 1.402**<br>(.22)   |
| Mid                  | 1.056<br>(.149)    | 1.062<br>(.145)    | 1.12<br>(.161)     | 1.023<br>(.147)     | .718**<br>(.104)  | 1.043<br>(.144)    |
| <b>LT experience</b> | 1.094*<br>(.054)   | 1.184***<br>(.058) | 1.104**<br>(.054)  | 1.348***<br>(.068)  | 1.174***<br>(.06) | 1.33***<br>(.066)  |
| <b>LT literacy</b>   | 1.083<br>(.293)    | 2.145***<br>(.592) | 1.826**<br>(.487)  | 5.435***<br>(1.396) | 1.797**<br>(.486) | 1.986***<br>(.527) |
| Observations         | 1407               | 1385               | 1401               | 1388                | 1350              | 1385               |
| Pseudo $R^2$         | .015               | .026               | .02                | .068                | .024              | .024               |

Note:

\*p<0.1; \*\*p<0.05; \*\*\*p<0.01

**Table S7 Odds Ratio for the frequency of use of GenAI chatbots.** Results from 6 different ordinal regression models, one per intent (columns). Standard Errors are reported between parentheses.

|                 | Dependent Variable: Chatbot User (Binary) |                      |                      |                      |                      |
|-----------------|-------------------------------------------|----------------------|----------------------|----------------------|----------------------|
|                 | (1)<br>Baseline                           | (2)<br>+SocioDemo    | (3)<br>+Edu          | (4)<br>+LT Exp       | (5)<br>+LT Lit       |
| Woman           | -0.771***<br>(0.122)                      | -0.835***<br>(0.133) | -0.863***<br>(0.133) | -0.790***<br>(0.137) | -0.690***<br>(0.142) |
| Marginal Effect | -0.117                                    | -0.114               | -0.117               | -0.101               | -0.083               |
| Pseudo $R^2$    | 0.023                                     | 0.116                | 0.124                | 0.169                | 0.218                |
| N               | 1,883                                     | 1,833                | 1,833                | 1,833                | 1,833                |

**Table S8 Sequential Decomposition: Gender Gap in GenAI Chatbot Adoption.** Logistic regression coefficients with standard errors in parentheses. Reference category: Man. Controls progressively added: (2) Sociodemographics: Age, Geography, Socioeconomic Status; (3) Education level (graduate vs non-graduate); (4) Language technology experience; (5) Language Technology literacy. \*\*\* $p < 0.01$ , \*\* $p < 0.05$ , \* $p < 0.1$

|                              | (1)<br>Baseline      | (2)<br>+Demo         | (3)<br>+Edu          | (4)<br>+LT Exp       | (5)<br>+LT Lit       |
|------------------------------|----------------------|----------------------|----------------------|----------------------|----------------------|
| <i>Information Retrieval</i> |                      |                      |                      |                      |                      |
| Female                       | -0.271***<br>(0.059) | -0.223***<br>(0.060) | -0.226***<br>(0.060) | -0.220***<br>(0.060) | -0.220***<br>(0.061) |
| AME                          | -0.271***<br>(0.059) | -0.223***<br>(0.060) | -0.226***<br>(0.060) | -0.220***<br>(0.060) | -0.220***<br>(0.061) |
| $R^2$                        | 0.015                | 0.033                | 0.033                | 0.034                | 0.034                |
| N                            | 1,446                | 1,407                | 1,407                | 1,407                | 1,407                |
| <i>Problem Solving</i>       |                      |                      |                      |                      |                      |
| Female                       | -0.419***<br>(0.056) | -0.415***<br>(0.058) | -0.414***<br>(0.058) | -0.397***<br>(0.058) | -0.376***<br>(0.058) |
| AME                          | -0.419***<br>(0.056) | -0.415***<br>(0.058) | -0.414***<br>(0.058) | -0.397***<br>(0.058) | -0.376***<br>(0.058) |
| $R^2$                        | 0.037                | 0.042                | 0.042                | 0.050                | 0.057                |
| N                            | 1,424                | 1,385                | 1,385                | 1,385                | 1,385                |
| <i>Learning</i>              |                      |                      |                      |                      |                      |
| Female                       | -0.328***<br>(0.055) | -0.342***<br>(0.056) | -0.338***<br>(0.056) | -0.329***<br>(0.057) | -0.312***<br>(0.057) |
| AME                          | -0.328***<br>(0.055) | -0.342***<br>(0.056) | -0.338***<br>(0.056) | -0.329***<br>(0.057) | -0.312***<br>(0.057) |
| $R^2$                        | 0.024                | 0.040                | 0.041                | 0.044                | 0.048                |
| N                            | 1,440                | 1,401                | 1,401                | 1,401                | 1,401                |
| <i>Content Creation</i>      |                      |                      |                      |                      |                      |
| Female                       | -0.136**<br>(0.060)  | -0.164***<br>(0.059) | -0.179***<br>(0.059) | -0.144**<br>(0.058)  | -0.097*<br>(0.058)   |
| AME                          | -0.136**<br>(0.060)  | -0.164***<br>(0.059) | -0.179***<br>(0.059) | -0.144**<br>(0.058)  | -0.097*<br>(0.058)   |
| $R^2$                        | 0.004                | 0.097                | 0.108                | 0.137                | 0.164                |
| N                            | 1,426                | 1,388                | 1,388                | 1,388                | 1,388                |
| <i>Leisure</i>               |                      |                      |                      |                      |                      |
| Female                       | -0.333***<br>(0.054) | -0.319***<br>(0.056) | -0.314***<br>(0.056) | -0.303***<br>(0.056) | -0.286***<br>(0.056) |
| AME                          | -0.333***<br>(0.054) | -0.319***<br>(0.056) | -0.314***<br>(0.056) | -0.303***<br>(0.056) | -0.286***<br>(0.056) |
| $R^2$                        | 0.026                | 0.035                | 0.037                | 0.040                | 0.045                |
| N                            | 1,388                | 1,350                | 1,350                | 1,350                | 1,350                |
| <i>Creativity</i>            |                      |                      |                      |                      |                      |
| Female                       | -0.194***<br>(0.057) | -0.194***<br>(0.058) | -0.191***<br>(0.058) | -0.161***<br>(0.057) | -0.140**<br>(0.058)  |
| AME                          | -0.194***<br>(0.057) | -0.194***<br>(0.058) | -0.191***<br>(0.058) | -0.161***<br>(0.057) | -0.140**<br>(0.058)  |
| $R^2$                        | 0.008                | 0.028                | 0.029                | 0.053                | 0.059                |
| N                            | 1,423                | 1,385                | 1,385                | 1,385                | 1,385                |

**Table S9 Sequential Decomposition by Intent Type: Gender Gap in GenAI Chatbot Frequency of Usage.** OLS regression coefficients with standard errors in parentheses. AME: Average Marginal Effect of being a Woman on usage frequency. Each panel shows the sequential decomposition for one intent type. Reference category: Man. Controls progressively added across columns. (2) Demo = Demographics (Age, Geography, Socioeconomic); (3) Edu = Education level (graduate vs non-graduate); (4) Language technology experience; (5) Language Technology literacy. \*\*\* $p < 0.01$ , \*\* $p < 0.05$ , \* $p < 0.1$
